# Supplementary material for: Token Merging: Your ViT But Faster
Source: arXiv:2210.09461 source file (2023-03-01)
Supplement: Supplementary file 1 [file sd_concept_and_quantitative.tex]

\begin{figure}[h]
\centering

\begin{minipage}{0.38\linewidth}{
    \centering
    \includegraphics[width=0.9\linewidth]{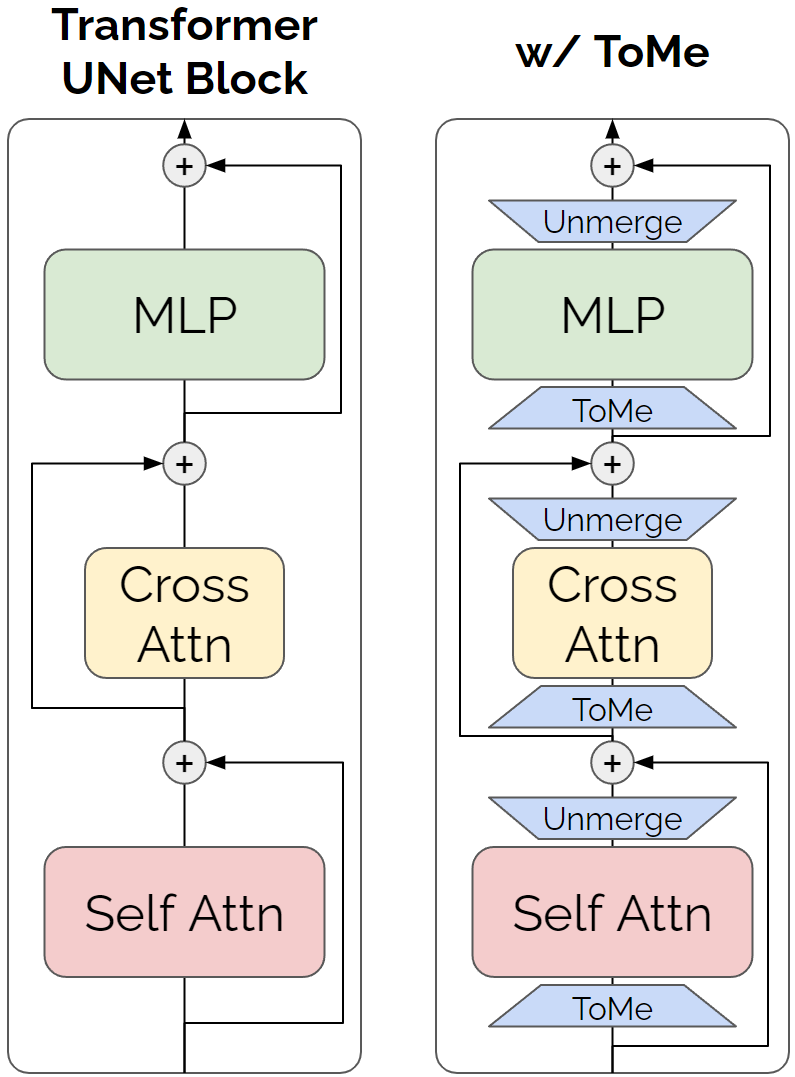}
    
    \captionof{figure}{\textbf{UNet w/ ToMe.} A visualization of ToMe applied to a transformer UNet block using the strategy discussed in Appendix~\ref{appendix:stable_diffusion_method}. }
    \label{fig:appendix_sd_block}
}\end{minipage}
\hspace{1em}
\begin{minipage}{0.58\linewidth}{
    \centering
    \tablestyle{4pt}{1.05}
    \begin{tabular}{y{40}x{20}|x{30}x{30}x{20}x{30}}
        Method & r\% & FID $\downarrow$ & s/im $\downarrow$ & bs $\uparrow$ & res $\uparrow$ \\
        \shline
        \gc{Baseline} & \gc{0} & \gc{33.29} & \gc{3.06} & \gc{7} & \gc{$1344^2$} \\[3pt]
        Pruning & 10 & 47.98 & 2.51 & 9 & $1536^2$ \\
        & 20 & 87.84 & 2.15 & 11 & $1664^2$ \\[3pt]
        \textbf{ToMe} & 10 & \textbf{33.14} & 2.60 & 8 & $1408^2$ \\
        & 20 & 33.53 & 2.29 & 11 & $1664^2$ \\
        & 30 & 33.60 & 2.11 & 14 & $1920^2$ \\
        & 40 & 34.67 & 1.81 & 19 & $2240^2$ \\
        & 50 & 38.95 & \textbf{1.53} & \textbf{27} & {$\mathbf{2624^2}$} \\
    \end{tabular}
    \captionof{table}{\textbf{ToMe applied to Stable Diffusion v1.5.} ToMe applied \textit{without training} as described in Appendix~\ref{appendix:stable_diffusion_method} for different token reduction percentages compared to the \gc{baseline} unmodified model and random token pruning. We report FID score \cite{fid}, seconds per image, max 512x512 img batch size, and max resolution with a batch size of 1. For each, we generate 2,000 512x512 images of ImageNet-1k classes (2 per class) using 50 PLMS \cite{plms} diffusion steps with a cfg scale of 7.5. Time per image is averaged over the 2,000 samples using a 4090 GPU and FID is computed between those 2,000 samples and 5,000 class-balanced ImageNet-1k val examples.}
    \label{tab:appendix_sd_results}
}\end{minipage}
\end{figure}
