# Supplementary material for: Token Merging: Your ViT But Faster
Source: arXiv:2210.09461 source file (2023-03-01)
Supplement: Supplementary file 2 [file sd_more_qualitative.tex]

\begin{figure}
    \centering
    \includegraphics[width=\linewidth]{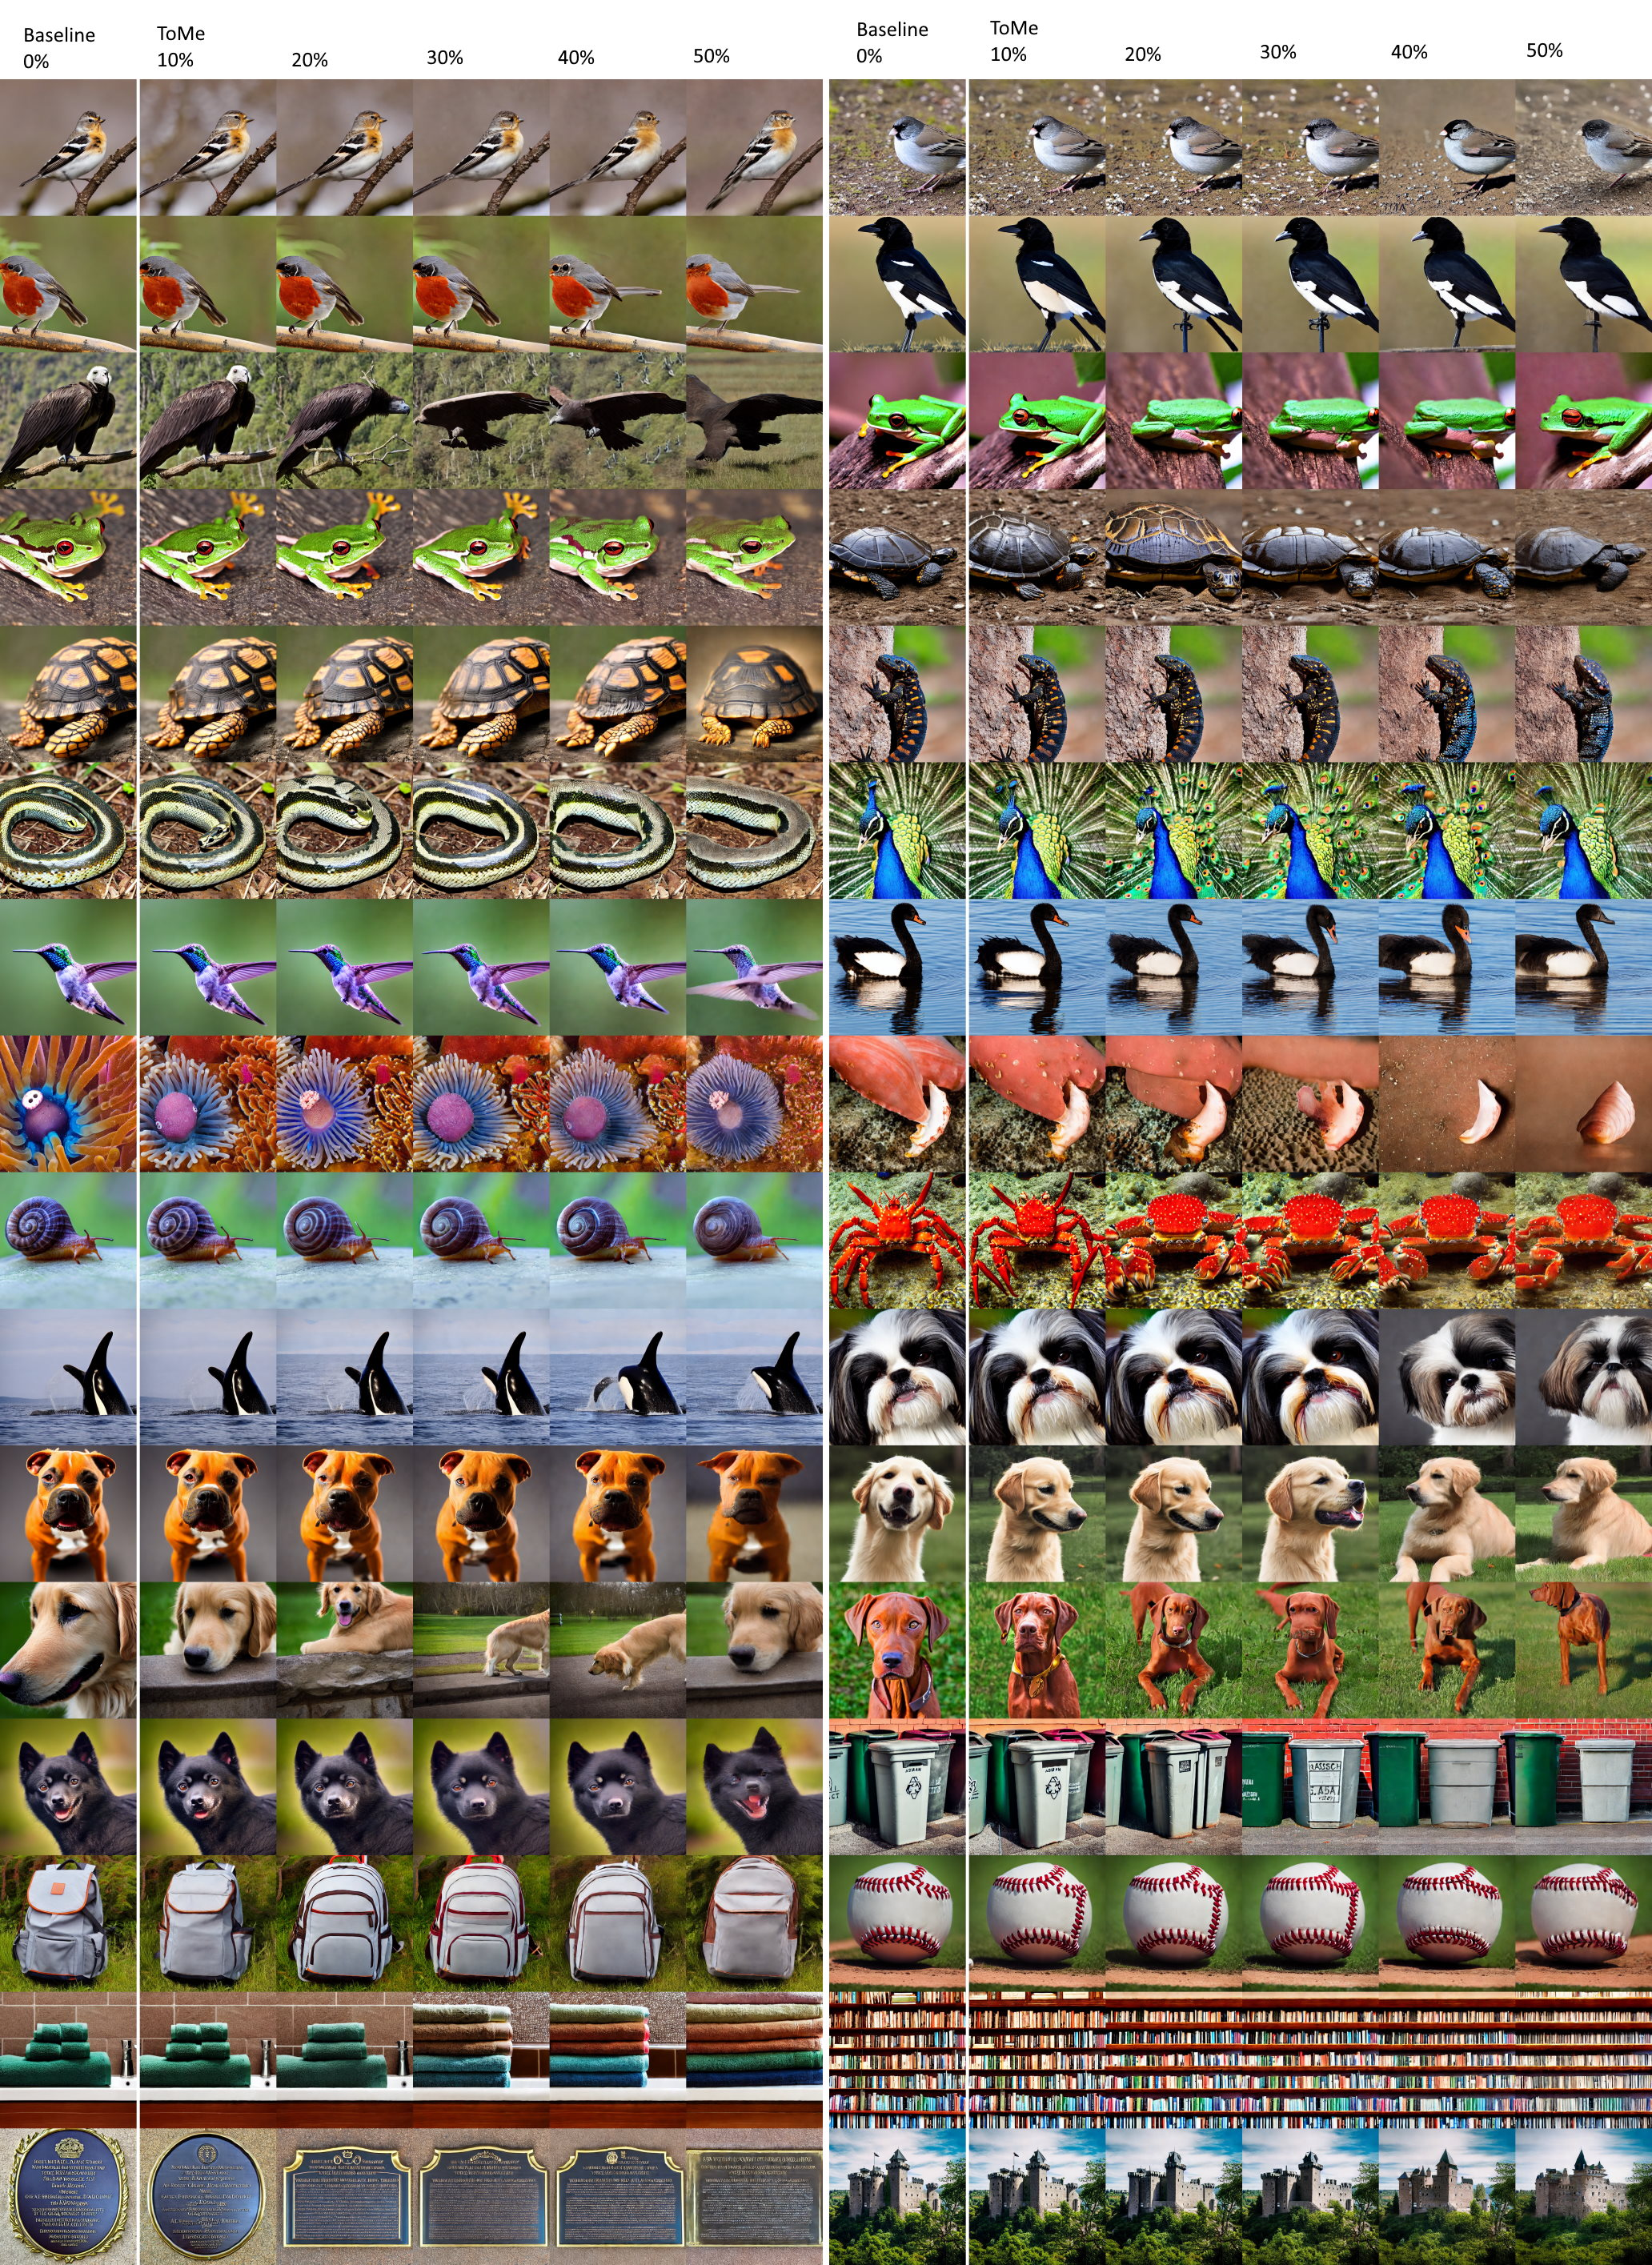}
    \caption{{\bf More Examples of Stable Diffusion with ToMe.} Visualization of the images generated with ToMe + SDv1.5 in Tab.~\ref{tab:appendix_sd_results}. For each image, the prompt is ``A high quality photograph of a $\langle x\rangle$.'' where $x$ is an ImageNet-1k class.}
    \label{fig:appendix_sd_more_qualitative}
\end{figure}
