# Supplementary material for: Token Merging: Your ViT But Faster
Source: arXiv:2210.09461 source file (2023-03-01)
Supplement: Supplementary file 3 [file sd_tome_vs_prune.tex]

\begin{figure}[h]

\centering
%#################################################
% ToMe
%#################################################
\subfloat[
    \textbf{ToMe} preserves image quality while merging up to half of all tokens, using \sfrac{1}{2} the time and \sfrac{1}{4} the memory.
    \label{fig:appendix_sd_comparison_tome}
]{
    \centering
    \begin{minipage}{0.47\linewidth}{
        \begin{center}
            \includegraphics[width=\linewidth]{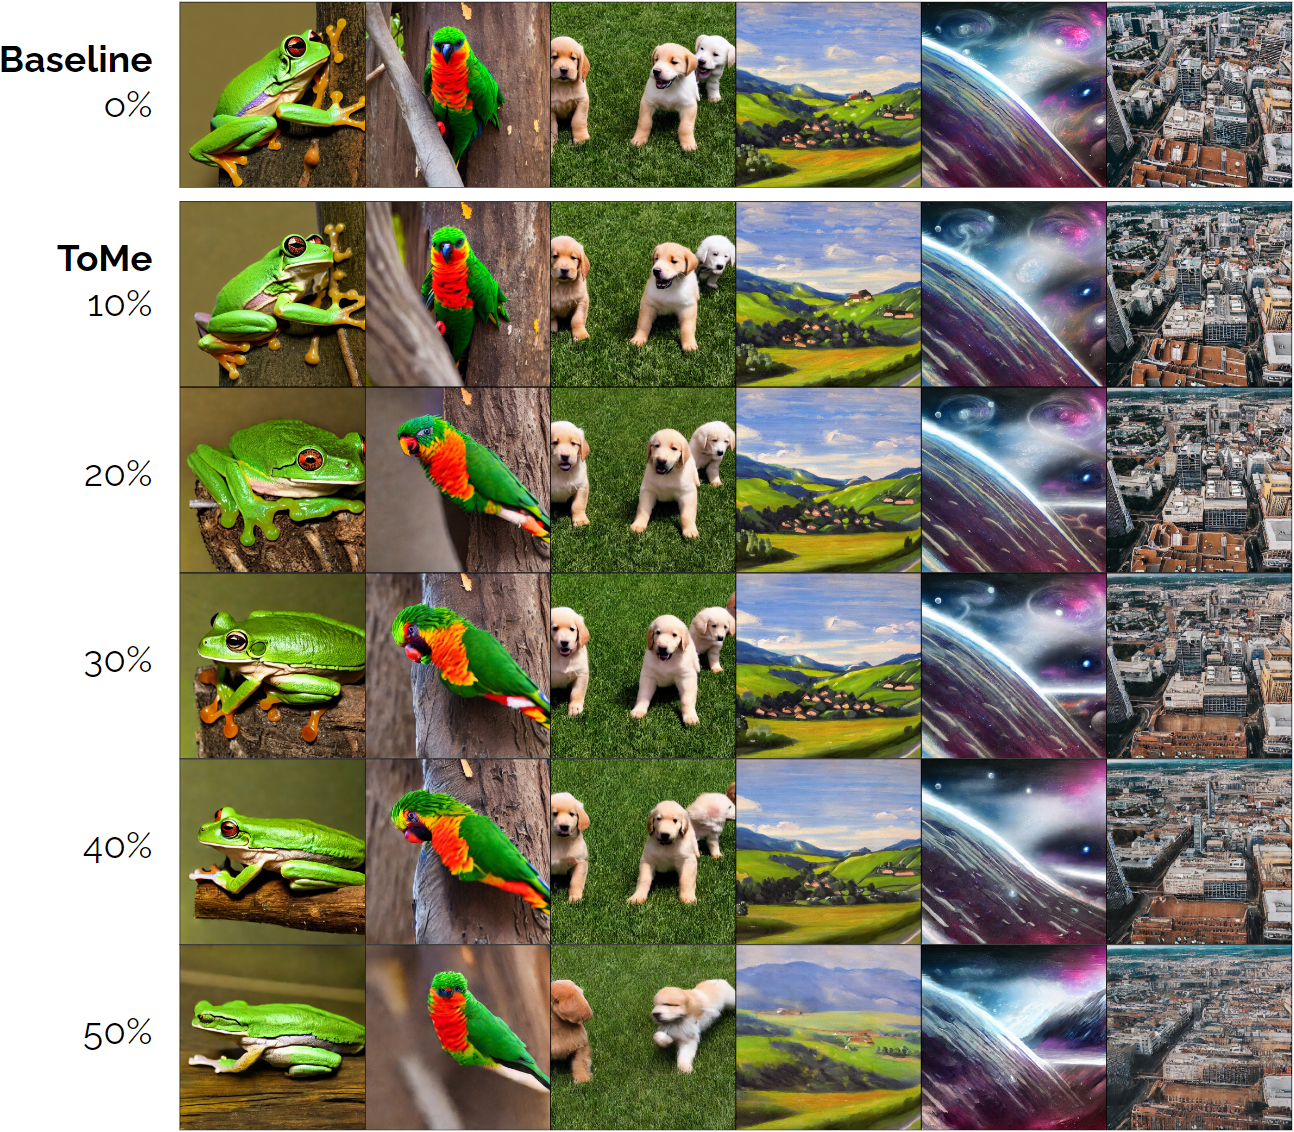}
    \end{center}}
    \end{minipage}
}
\hspace{1em}
%#################################################
% Pruning
%#################################################
\subfloat[
    \textbf{Pruning} tokens doesn't leave enough information to diffuse the image, resulting in brown blobs.
    \label{fig:appendix_sd_comparison_pruning}
]{
    \centering
    \begin{minipage}{0.47\linewidth}{
        \begin{center}
            \includegraphics[width=\linewidth]{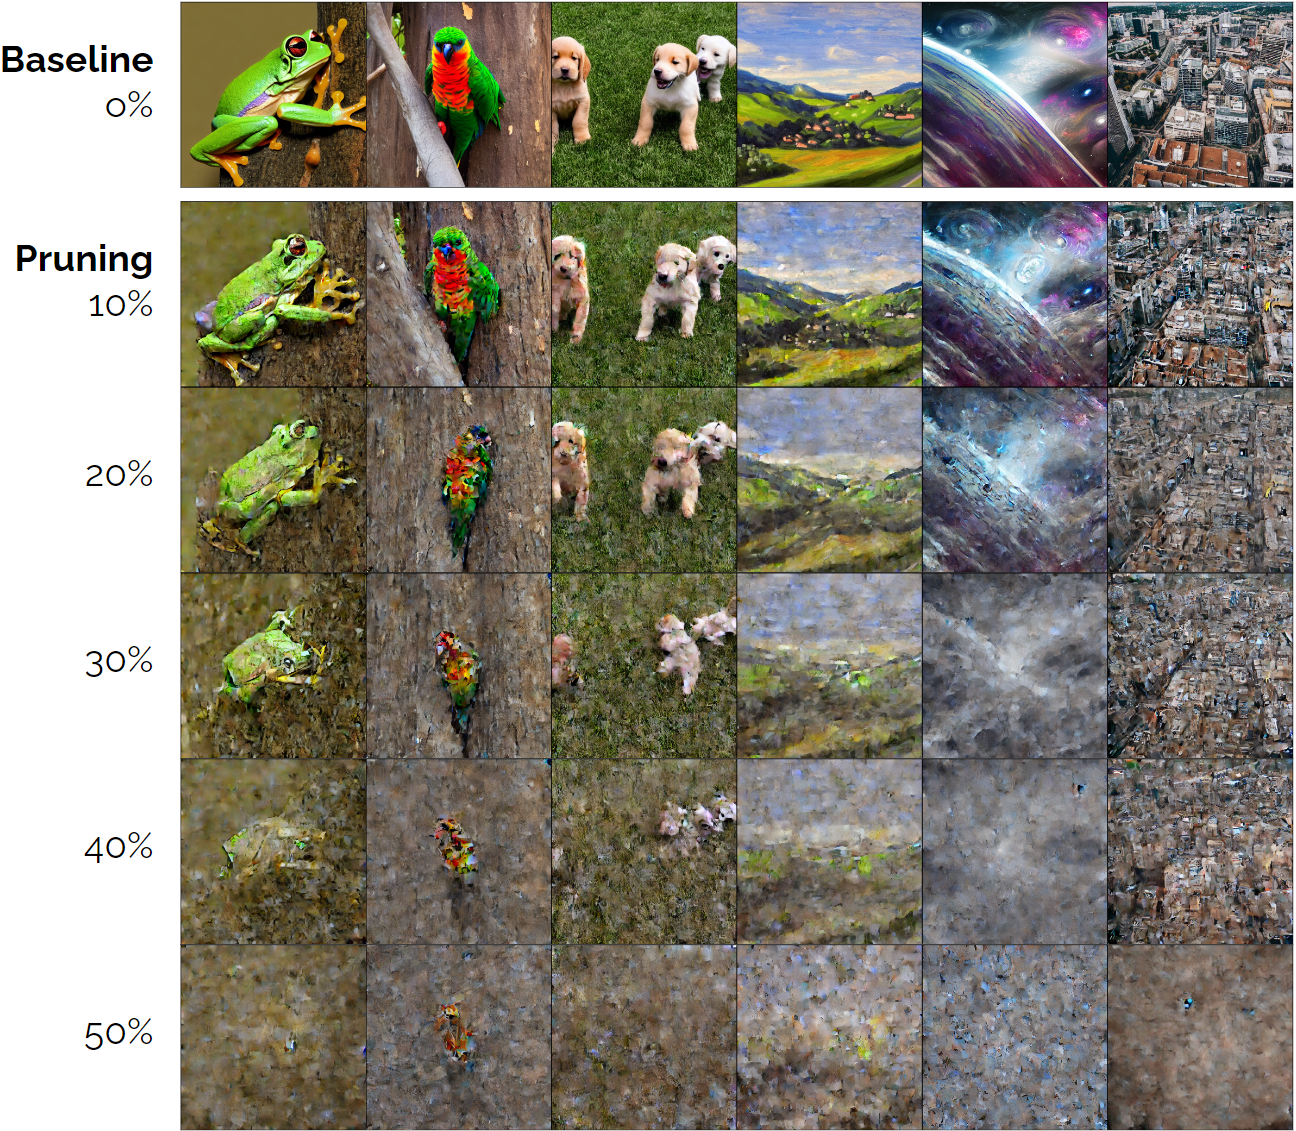}
    \end{center}}
    \end{minipage}
}
%#################################################
\caption{\textbf{ToMe vs. Pruning on Stable Diffusion.} ToMe and random token pruning applied to Stable Diffusion v1.5 with the same settings as Tab.~\ref{tab:appendix_sd_results}.}
\label{fig:appendix_sd_comparison}
\end{figure}
%##################################################################################################
